# Supplementary material for: Shedding light on charmonium
Source: arXiv:2312.02604 ancillary file (2023-12-05)
Supplement: Supplementary file 1 [file supplementary.pdf]

# Supplementary material to “Shedding light on charmonium”: a compilation of decay widths

Zhiguo Wang,<sup>1</sup> Meijian Li,<sup>2,\*</sup> Yang Li,<sup>1</sup> and James P. Vary<sup>3</sup>

<sup>1</sup>*Department of Modern Physics, University of Science and Technology of China, Hefei 230026, China*

<sup>2</sup>*Instituto Galego de Física de Altas Enerxías (IGFAE),  
Universidade de Santiago de Compostela, E-15782 Galicia, Spain*

<sup>3</sup>*Department of Physics and Astronomy, Iowa State University, Ames, Iowa 50011*

We provide in Table I a compilation experimental measurements and selected theoretical predictions of the E1 decay widths for charmonium, as supplementary to Figures presented in the paper.

TABLE I. A compilation of experimental measurements and selected theoretical predictions of the E1 decay widths for charmonium. The uncertainties have been combined in quadrature. Results not put in the table due to space limit:

| $\Gamma_{A \rightarrow B+\gamma}$ (keV) | Experiments      |              |              | BLFQ             | Lattice     |              |              | GI model |
|-----------------------------------------|------------------|--------------|--------------|------------------|-------------|--------------|--------------|----------|
|                                         | PDG [1]          | BESIII       | CLEO         | This work        | Chen’11 [2] | Dudek’09 [3] | Dudek’06 [4] | [5]      |
| $\chi_{c0}(1P) \rightarrow J/\psi(1S)$  | <b>151(10)</b>   | 27(233)[6]   | 216(33)[7]   | <b>162(16)</b>   | 85(7)       | 199(6)       | 232(41)      | 114      |
| $\psi(2S) \rightarrow \chi_{c0}(1P)$    | <b>28.8(1.0)</b> | 27.6(1.2)[6] | 27.1(1.6)[8] | <b>22(5)</b>     | —           | 26(11)       | —            | 26       |
| $\psi(3770) \rightarrow \chi_{c0}(1P)$  | <b>188(18)</b>   | 182(20)[9]   | 199(26)[10]  | <b>211(24)</b>   | —           | 265(66)      | —            | 213      |
| $\chi_{c0}(2P) \rightarrow J/\psi(1S)$  | —                | —            | —            | <b>0.6(4.5)</b>  | —           | —            | —            | 1.3      |
| $\chi_{c0}(2P) \rightarrow \psi(2S)$    | —                | —            | —            | <b>199(26)</b>   | —           | —            | —            | 135      |
| $\chi_{c0}(2P) \rightarrow \psi(3770)$  | —                | —            | —            | <b>52.9(1.5)</b> | —           | —            | —            | 51       |
| $h_c(1P) \rightarrow \eta_c(1S)$        | <b>445(164)</b>  | 445(166)[11] | 437(167)[12] | <b>489(85)</b>   | 234(12)     | —            | 601(55)      | 352      |
| $\eta_c(2S) \rightarrow h_c(1P)$        | —                | —            | —            | <b>26.4(1.1)</b> | —           | —            | —            | 36       |

| $\Gamma_{A \rightarrow B+\gamma}$ (keV) | Experiments  |              |              | Lattice         |           |                   |
|-----------------------------------------|--------------|--------------|--------------|-----------------|-----------|-------------------|
|                                         | CBAL’86 [13] | CNTR’77 [14] | MRK1’76 [15] | Delaney’23 [16] | Li’21[17] | Becirevic’12 [18] |
| $\chi_{c0}(1P) \rightarrow J/\psi(1S)$  | —            | —            | —            | 204(5)          | 180(96)   | —                 |
| $\psi(2S) \rightarrow \chi_{c0}(1P)$    | 29.1(2.9)    | 21(7)        | 22(8)        | —               | —         | —                 |
| $h_c(1P) \rightarrow \eta_c(1S)$        | —            | —            | —            | —               | —         | 720(50)(20)       |

\* [meijian.li@usc.es](mailto:meijian.li@usc.es)

- [1] R. L. Workman *et al.* [Particle Data Group], PTEP **2022**, 083C01 (2022) doi:10.1093/ptep/ptac097
- [2] Y. Chen, D. C. Du, B. Z. Guo, N. Li, C. Liu, H. Liu, Y. B. Liu, J. P. Ma, X. F. Meng and Z. Y. Niu, *et al.* Phys. Rev. D **84**, 034503 (2011) doi:10.1103/PhysRevD.84.034503 [arXiv:1104.2655 [hep-lat]].
- [3] J. J. Dudek, R. Edwards and C. E. Thomas, Phys. Rev. D **79**, 094504 (2009) doi:10.1103/PhysRevD.79.094504 [arXiv:0902.2241 [hep-ph]].
- [4] J. J. Dudek, R. G. Edwards and D. G. Richards, Phys. Rev. D **73**, 074507 (2006) doi:10.1103/PhysRevD.73.074507 [arXiv:hep-ph/0601137 [hep-ph]].
- [5] T. Barnes, S. Godfrey and E. S. Swanson, Phys. Rev. D **72**, 054026 (2005) doi:10.1103/PhysRevD.72.054026 [arXiv:hep-ph/0505002 [hep-ph]].
- [6] M. Ablikim *et al.* [BESIII], Phys. Rev. D **96**, no.3, 032001 (2017) doi:10.1103/PhysRevD.96.032001 [arXiv:1703.00077 [hep-ex]].
- [7] N. E. Adam *et al.* [CLEO], Phys. Rev. Lett. **94**, 232002 (2005) doi:10.1103/PhysRevLett.94.232002 [arXiv:hep-ex/0503028 [hep-ex]].
- [8] S. B. Athar *et al.* [CLEO], Phys. Rev. D **70**, 112002 (2004) doi:10.1103/PhysRevD.70.112002 [arXiv:hep-ex/0408133 [hep-ex]].
- [9] M. Ablikim *et al.* [BESIII], Phys. Lett. B **753**, 103-109 (2016) doi:10.1016/j.physletb.2015.11.074 [arXiv:1511.01203 [hep-ex]].
- [10] R. A. Briere *et al.* [CLEO], Phys. Rev. D **74**, 031106 (2006) doi:10.1103/PhysRevD.74.031106 [arXiv:hep-ex/0605070 [hep-ex]].

- [11] M. Ablikim *et al.* [BESIII], Phys. Rev. D **106**, no.7, 072007 (2022) doi:10.1103/PhysRevD.106.072007 [arXiv:2204.09413 [hep-ex]].
- [12] S. Dobbs *et al.* [CLEO], Phys. Rev. Lett. **101**, 182003 (2008) doi:10.1103/PhysRevLett.101.182003 [arXiv:0805.4599 [hep-ex]].
- [13] J. Gaiser, E. D. Bloom, F. Bulos, G. Godfrey, C. M. Kiesling, W. S. Lockman, M. Oreglia, D. L. Scharre, C. Edwards and R. Partridge, *et al.* Phys. Rev. D **34**, 711 (1986) doi:10.1103/PhysRevD.34.711
- [14] C. J. Biddick, T. H. Burnett, G. E. Masek, E. S. Miller, J. G. Smith, J. P. Stronski, M. K. Sullivan, W. Vernon, D. H. Badtke and B. A. Barnett, *et al.* Phys. Rev. Lett. **38**, 1324 (1977) doi:10.1103/PhysRevLett.38.1324
- [15] J. S. Whitaker, W. M. Tanenbaum, G. S. Abrams, M. S. Alam, A. Boyarski, M. Breidenbach, W. Chinowsky, R. DeVoe, G. J. Feldman and C. E. Friedberg, *et al.* Phys. Rev. Lett. **37**, 1596 (1976) doi:10.1103/PhysRevLett.37.1596
- [16] J. Delaney, C. E. Thomas and S. M. Ryan, [arXiv:2301.08213 [hep-lat]].
- [17] N. Li, C. C. Liu and Y. J. Wu, EPL **133**, no.1, 11001 (2021) doi:10.1209/0295-5075/133/11001
- [18] D. Becirevic and F. Sanfilippo, JHEP **01**, 028 (2013) doi:10.1007/JHEP01(2013)028 [arXiv:1206.1445 [hep-lat]].
